# Supplementary material for: Machine learning on DNA-encoded libraries: A new paradigm for hit-finding
Source: arXiv:2002.02530 source file (2020-01-31)
Supplement: Supplementary file 1 [file supporting_info.tex]

\documentclass{article}

\usepackage[utf8]{inputenc}
\usepackage[T1]{fontenc}
\usepackage{booktabs}
\usepackage{siunitx}
\usepackage{makecell}
\usepackage{textcomp}
\usepackage[table]{xcolor}
\usepackage{colortbl}

% alternating table rows
\definecolor{lightgray}{gray}{0.9}

\begin{document}

\end{document}
